# Supplementary material for: Staged Contact-Aware Global Human Motion Forecasting
Source: arXiv:2309.08947 source file (2023-09-16)
Supplement: Supplementary file 1 [file intro.tex]

We supplement the main paper submission with additional details and qualitative results. The supplementary material is organized according to the following table of contents.
