# Supplementary material for: Staged Contact-Aware Global Human Motion Forecasting
Source: arXiv:2309.08947 source file (2023-09-16)
Supplement: Supplementary file 2 [file mocap_suppmat.tex]

\begin{table}[!htp]
\centering

\scriptsize
\begin{tabular}{l|ccc}
\hline
\textbf{} & \multicolumn{3}{c}{\textbf{Global Error}} \\
\textbf{Models} &\textbf{1s} &\textbf{2s} &\textbf{3s} \\
\hline
LTD~\cite{mao2019learning} &  0.480& 0.869& 1.181\\
HRI~\cite{mao2020history} & 0.503 & 0.932 & 1.422 \\
SocialPool~\cite{Adeli2020SociallyAC} & {---} & {---} & {---}\\
MR-Trans~\cite{Wang2021MultiPerson3M}& 0.456 & 0.840 & 1.110 \\

SoMoFormer~\cite{vendrow2022somoformer}& \textbf{0.420} & \textbf{0.800} & \textbf{1.060} \\

Mao \etal~\cite{mao2022contact}~\textit{w/ pred contact}& {0.485} & {1.24} & {2.01}\\
%\hline
\model~\textit{w/ pred contact} & 0.441 & 0.851 & 1.145 \\ 
\hline

\end{tabular}
\caption{Global error in meters on CMU-Mocap dataset. \FG{these numbers appear nowhere in the somoformer paper, right? GIven the premises on that paper and the proposed iteration of this section, I'd suggest you remove this table from the supp mat. It's not helping the message, it's not formally due, and (as you claim) it might not be even correct. Altogether, it's creating more issues than it resolves.}}
\label{tab: mocap}
\end{table}
